# Supplementary material for: Rethinking Structure Learning For Graph Neural Networks
Source: arXiv:2411.07672 source file (2024-11-12)
Supplement: Supplementary file 1 [file proof_old.tex]

\section{Proof of Theorem}

\yilun{Try Bernoulli sampling}

\yilun{Try state transfer to prove inductively}

\yilun{Central Limit Theorem to support why GCN better than MLP in homophily graphs}

\textcolor{red}{New Solution}
\begin{equation}
    \begin{split}
        I(y;h') - I(y;h)
        &=\bigl[H(h')-H(h'|y)\bigr]-\bigl[H(h)-H(h|y)\bigr] \\
        &=\bigl[H(h')-H(h)\bigr]-\bigl[H(h|y)-H(h'|y)\bigr] \\
    \end{split}
\end{equation}

First term denotes the differences of entropy, which can be expressed as
\begin{equation}
    \begin{split}
        \bigl[H(h')-H(h)\bigr]
        &=-\int_{h'} p(h')log\ p(h') dh'+\int_{h} p(h)log\ p(h) dh \\
        &=-\int_{h'} \left[ \sum_y p(y)p(h'|y) \right] log\ \left[ \sum_y p(y)p(h'|y) \right] dh' \\
        &+\int_{h} \left[ \sum_y p(y)p(h|y) \right]log\ \left[ \sum_y p(y)p(h|y) \right] dh \\
        &=-\int_{h'} \left[ \sum_y p(y)p(h'|y) \right] log\ \left[ \sum_y p(y)p(h'|y) \right] dh' \\
        &+\int_{h} \left[ \sum_y p(y)p(h|y) \right]log\ \left[ \sum_y p(y)p(h|y) \right] dh \\
    \end{split}
\end{equation}


\textcolor{red}{Old Solution}

To analyze the performance of through CSBM models, we consider the mutual information between the aggregated features $\bd{H}$ with labels $\bd{Y}$. Unlike \cite{} that only consider inter-class distances or intra-class distances, mutual information considers both the distances and is scale invariant, which better aligns with the model performance. The difference of the mutual information between new graph $\mathcal{G}$ and original graph $\mathcal{G}'$ can be expressed as (We only consider one dimension of $\bd{h}$ there for simplicity):
\begin{equation}
    \begin{split}
        I(y;h') - I(y;h) 
        &=\left(H(y)-H(y|h')\right)-\left(H(y)-H(y|h)\right) \\
        &=H(y|h) - H(y|h') \\
        &= \sum_{y\in\mathcal{Y}}\left[
        -\int_{h} p(y,h)\text{log}\ p(y|h) dh
        +\int_{h'} p(y,h')\text{log}\ p(y|h') dh'\right]
    \end{split}
\end{equation}
Suppose the aggregated node features $h$ of $\mathcal{G}$ of class $y$ follow a class-wised Gaussian distribution $N_y$ ( and $N_y'$ for $\mathcal{G}'$). Then we can express the joint probability $p(y,h)$ and conditional probability $p(y|h)$ as:
\begin{equation}
    \begin{split}
        p(y,h) &= p(y)p(h|y) = p(y)p(N_y=h)\\
        p(y|h) &= \frac{p(y,h)}{p(h)} = \frac{p(y)p(h|y)}{\sum_{y\in\mathcal{Y}}p(y)p(h|y)} = \frac{p(y)p(N_y=h)}{\sum_{y\in\mathcal{Y}}p(y)p(N_y=h)}
    \end{split}
\end{equation}
Similarly, we can get the expression of $p(y,h')$ and $p(y|h')$ as above. Then, we have
\begin{equation}
    \begin{split}
        I(y;h) - I(y;h')
        &= \sum_{y\in\mathcal{Y}}p(y)\left[
        \int_{h} p(N_y=h)\text{log}\ \frac{p(y)p(N_y=h)}{\sum_{y\in\mathcal{Y}}p(y)p(N_y=h)} dh \right. \\
        &\left. -\int_{h'} p(N'_y=h')\text{log}\ \frac{p(y)p(N'_y=h')}{\sum_{y\in\mathcal{Y}}p(y)p(N'_y=h')} dh'\right] \\
        &= \sum_{y\in\mathcal{Y}}p(y)\left[
        \int_{h} \left( p(N_y=h)\text{log}\ \frac{p(y)p(N_y=h)}{\sum_{y\in\mathcal{Y}}p(y)p(N_y=h)} \right. \right. \\
        &\left.\left. - p(N'_y=h)\text{log}\ \frac{p(y)p(N'_y=h)}{\sum_{y\in\mathcal{Y}}p(y)p(N'_y=h)} dh\right)\right] \\
        &= \sum_{y\in\mathcal{Y}}p(y)\int_{h}
        \left(p(N_y'=h)-p(N_y=h)\right)p(h)dh + \sum_{y\in\mathcal{Y}}p(y)\left[H(N_y')-H(N_y)\right] \\
    \end{split}
\end{equation}

The first term is similar as "error rate" in Bayes classifier and the second term is the uncertainty of the distribution of the samples in each class.

Let's consider the first term,
\begin{equation}
    \begin{split}
        &\sum_{y\in\mathcal{Y}}p(y)\int_{h}
        \left(p(N_y'=h)-p(N_y=h)\right)p(h)dh \\
        &=\sum_{y\in\mathcal{Y}}p(y)\int_{h}
        \left(p(N_y'=h)-p(N_y=h)\right)\sum_{z\in\mathcal{Y}}p(z)p(N_z=h)dh\\
        &=\sum_{y\in\mathcal{Y}}\sum_{z\in\mathcal{Y}}p(y)p(z)\int_{h}
        \left(p(N_y'=h)-p(N_y=h)\right)p(N_z=h)dh\\
        &=\sum_{y\in\mathcal{Y}}\sum_{z\in\mathcal{Y}}p(y)p(z)\int_{h}
        p(N_y'=h)p(N_z=h)dh-p(N_y=h)p(N_z=h)dh\\
        &=\sum_{y\in\mathcal{Y}}\sum_{z\in\mathcal{Y}}p(y)p(z)\left[
        p(N_z=N_y') - p(N_z=N_y)
        \right] \\
    \end{split}
\end{equation}

and the second term,
\begin{equation}
    \begin{split}
        \sum_{y\in\mathcal{Y}}p(y)\left[H(N_y')-H(N_y)\right] 
        =\sum_{y\in\mathcal{Y}}p(y)\left[\frac{1}{2}\ln{\left(\frac{\sigma'^2_y}{\sigma^2_y}\right)}\right]
    \end{split}
\end{equation}

Combine these two terms, we have
\begin{equation}\label{eq:MI_diff_final}
    \begin{split}
    % \resizebox{1\hsize}{!}{$
        I(y;h) - I(y;h') = 
        \sum_{y\in\mathcal{Y}}\sum_{z\in\mathcal{Y}}p(y)p(z)\left[
        p(N_z=N_y') - p(N_z=N_y)
        \right]
        + \sum_{y\in\mathcal{Y}}p(y)\left[\frac{1}{2}\ln{\left(\frac{\sigma'^2_y}{\sigma^2_y}\right)}\right]
    % $}
    \end{split}
\end{equation}

In order to inspect the differences of these mutual information, in the next, we show how to get the distribution of the aggregated features $N_y$ and $N'_y$ of $\mathcal{G}$ and $\mathcal{G}'$ respectively.

For the original graph $\mathcal{G}$, we have the feature of node $u$ with class $y$ as $x_u\sim N(\mu_y,\sigma_y^2)$. On the other hand, for the new graph $\mathcal{G}'$, we first consider the distribution of class labels of the neighbors. Specifically, in a new graph $\mathcal{G}'$ that uses features to rewrite the topology with a threshold $\delta$, the probability the node $u$ with class $y$ connect with nodes with class $k$ is given by
\begin{equation}
    p(k|y) = r_{y,k} = \frac{p(x_y x_k>\delta)}{\sum_{z\in\mathcal{C}}p(x_y x_z>\delta)}
\end{equation}
Then we have the aggregated features in new graph $\mathcal{G}'$
\begin{equation}
    h'_u = \sum_{k\in\mathcal{Y}} r_{y,k} x_k \sim N'_y(\mu'_y,\sigma'^2_y)
\end{equation}
where the $\mu'_y$ and $\sigma'^2_y$ is given by
\begin{equation}
    \begin{split}
        \mu'_y &=\frac{\sum_{k\in\mathcal{Y}}p(x_y x_k>\delta)\mu_k}{\sum_{k\in\mathcal{Y}}p(x_y x_k>\delta)} \\
        \sigma'^2_y &= \frac{\sum_{k\in\mathcal{Y}}p(x_y x_k>\delta)\sigma^2_k}{\sum_{k\in\mathcal{Y}}p(x_y x_k>\delta)} \\
    \end{split}
\end{equation}

Then we take back to the first term in Eq. (\ref{eq:MI_diff_final})
\begin{equation}
    \begin{split}
        &\sum_{y\in\mathcal{Y}}\sum_{z\in\mathcal{Y}}p(y)p(z)\left[
        p(N_z=N_y') - p(N_z=N_y)
        \right] \\
        &=\sum_{y\in\mathcal{Y}}\sum_{z\in\mathcal{Y}}p(y)p(z)
        \left[\frac{1}{\sqrt{2\pi({\sigma'}_y^2+\sigma_z^2)}}\text{exp}\left(-\frac{(\mu_y'-\mu_z)^2}{2({\sigma'}_y^2+\sigma_z^2)}\right)-\frac{1}{\sqrt{2\pi(\sigma^2_y+\sigma_z^2)}}\text{exp}\left(-\frac{(\mu_y-\mu_z)^2}{2({\sigma}_y^2+\sigma_z^2)}\right)\right] \\
    \end{split}
\end{equation}

To derive the sign of this equality, we have

\begin{equation}
    \begin{split}
        &\sum_{y\in\mathcal{Y}}\sum_{z\in\mathcal{Y}}p(y)p(z)
        \left[\frac{1}{\sqrt{2\pi({\sigma'}_y^2+\sigma_z^2)}}\text{exp}\left(-\frac{(\mu_y'-\mu_z)^2}{2({\sigma'}_y^2+\sigma_z^2)}\right)\right]\\
        &\ge \sum_{y\in\mathcal{Y}}\sum_{z\in\mathcal{Y}}p(y)p(z)\sum_{k\in\mathcal{Y}}p(k|y)\left[\frac{1}{\sqrt{2\pi({\sigma}_y^2+\sigma_z^2)}}\text{exp}\left(-\frac{(\mu_y'-\mu_z)^2}{2({\sigma}_y^2+\sigma_z^2)}\right)\right] \\
        &= \sum_{k\in\mathcal{Y}}\sum_{z\in\mathcal{Y}}p(k)p(z)\left[\frac{1}{\sqrt{2\pi({\sigma}_k^2+\sigma_z^2)}}\text{exp}\left(-\frac{(\mu_y'-\mu_z)^2}{2({\sigma}_k^2+\sigma_z^2)}\right)\right] \\
        &= \sum_{y\in\mathcal{Y}}\sum_{z\in\mathcal{Y}}p(y)p(z)\left[\frac{1}{\sqrt{2\pi({\sigma}_y^2+\sigma_z^2)}}\text{exp}\left(-\frac{(\mu_y'-\mu_z)^2}{2({\sigma}_y^2+\sigma_z^2)}\right)\right] \\
        & \color{red}{\text{Not a rigorous result because the convex is unknown... Only verified by parts of numerical results }} \\
        &\ge \sum_{y\in\mathcal{Y}}\sum_{z\in\mathcal{Y}}p(y)p(z)\sum_{k\in\mathcal{Y}}p(k|y)\left[\frac{1}{\sqrt{2\pi({\sigma}_y^2+\sigma_z^2)}}\text{exp}\left(-\frac{(\mu_k-\mu_z)^2}{2({\sigma}_y^2+\sigma_z^2)}\right)\right] \\
        &= \sum_{y\in\mathcal{Y}}\sum_{z\in\mathcal{Y}}p(y)p(z)\left[\frac{1}{\sqrt{2\pi({\sigma}_y^2+\sigma_z^2)}}\text{exp}\left(-\frac{(\mu_y-\mu_z)^2}{2({\sigma}_y^2+\sigma_z^2)}\right)\right] \\
    \end{split}
\end{equation}
\textcolor{blue}{(Split into 2 steps to avoid symbol conflict)}

and 

\begin{equation}
    \begin{split}
        \text{exp}\left(-\frac{(\mu_y'-\mu_z)^2}{2({\sigma'}_y^2+\sigma_z^2)}\right)
        &=\text{exp}\left(-\frac{(\mu_y'-\mu_z)^2}{2\left(\sum_{k\in\mathcal{Y}}p(k|y)+\sigma_z^2\right)}\right)\\
        &\le\text{exp}\left(-\frac{(\mu_y'-\mu_z)^2}{2\left(\sum_{k\in\mathcal{Y}}p(k|y)+\sigma_z^2\right)}\right)\\
    \end{split}
\end{equation}

then for the second term in Eq. (\ref{eq:MI_diff_final})
\begin{equation}
    \begin{split}
        \sum_{y\in\mathcal{Y}}p(y)\left[\frac{1}{2}\ln{\left(\frac{\sigma'^2_y}{\sigma^2_y}\right)}\right]
        &=\sum_{y\in\mathcal{Y}}p(y)\left[\frac{1}{2}\ln{\left(\frac{\sum_{k\in\mathcal{Y}}r_{y,k}\sigma_k^2}{\sigma^2_y}\right)}\right] \\
        &=\sum_{y\in\mathcal{Y}}p(y)\left[\frac{1}{2}\ln{\left(\frac{\sum_{k\in\mathcal{Y}}p(k|y)\sigma_k^2}{\sigma^2_y}\right)}\right] \\
        &\ge \frac{1}{2}\sum_{y\in\mathcal{Y}}p(y)\left[\sum_{k\in\mathcal{Y}}p(k|y)\ln{(\sigma_k^2})-\ln{(\sigma^2_y)}\right] \\
        % &= \frac{1}{2}\sum_{y\in\mathcal{Y}}p(y)\left[\sum_{k\in\mathcal{Y}}p(k,y)p(y)^{-1}\ln{(\sigma_k^2})-\ln{(\sigma^2_y)}\right] \\
        % &= \frac{1}{2}\left[\sum_{y\in\mathcal{Y}}\sum_{k\in\mathcal{Y}}p(k,y)\ln{(\sigma_k^2}) - \sum_{y\in\mathcal{Y}}p(y)\ln(\sigma_y^2) \right] \\
        &= \frac{1}{2}\left[\sum_{k\in\mathcal{Y}}p(k)\ln{(\sigma_k^2}) - \sum_{y\in\mathcal{Y}}p(y)\ln(\sigma_y^2) \right] \\
        &= 0
    \end{split}
\end{equation}

Combine these two inequalities, finally we have 
\begin{equation}
    I(y;h) - I(y;h')\ge 0
\end{equation}
